# Supplementary material for: MADField: Multi-fidelity Amortized Density Field for Adsorption in Nanoporous Materials
Source: arXiv:2606.21284 source file (2026-07-01)
Supplement: Supplementary file 1 [file cDFT_warmstart_appendix.tex]

\begin{table}[t]
\caption{
\textbf{Iteration speedup by external-potential well-depth regime.}
\method{} warm-start consistently reduces Picard iterations, with larger gains on deeper potential wells.
}
\label{tab:warmstart_iter}
\footnotesize
\centering
\begin{tabular}{lccc}
\toprule
Metric & Shallow & Moderate & Deep \\
\midrule
Cold-start mean iter. & 241.6 & 349.4 & 445.3 \\
Warm-start mean iter. & 138.5 & 169.3 & 209.6 \\
\textbf{Iteration speedup} & \textbf{1.74$\times$} & \textbf{2.06$\times$} & \textbf{2.12$\times$} \\
\bottomrule
\end{tabular}
\end{table}
